# Supplementary material for: Causal Discovery from Temporal Data: An Overview and New Perspectives
Source: arXiv:2303.10112 source file (2023-08-03)
Supplement: Supplementary file 1 [file Appendix.tex]

% \appendix

% \section{Appendix}
% \subsection{Subsect}
% ...
